# Supplementary material for: In-situ local imaging of ferromagnetism and superconductivity in RbEuFe$_4$As$_4$
Source: arXiv:2407.11332 source file (2024-07-16)
Supplement: Supplementary file 1 [file SI_Nano_Lett.pdf]

# Supporting Information: In-situ local imaging of ferromagnetism and superconductivity in $RbEuFe_4As_4$

Huiyuan Man,[*,†,‡] Yusuke Iguchi,[†,¶] Jin-Ke Bao,[§] Duck Young Chung,[§] and Mercouri G. Kanatzidis[§,‖]

†*Geballe Laboratory for Advanced Materials, Stanford University, Stanford, CA 94305, USA*

‡*Stanford Nano Shared Facilities, Stanford University, Stanford, CA 94305, USA*

¶*Stanford Institute for Materials and Energy Sciences, SLAC National Accelerator Laboratory, Menlo Park, California 94025, USA*

§*Materials Science Division, Argonne National Laboratory, Argonne, Illinois 60439, USA*

‖*Department of Chemistry, Northwestern University, Evanston, Illinois 60208, USA*

E-mail: huiyuan653@gmail.com

## Supporting Note 1: Susceptometry and magnetometry scans

Figure S2 shows the scans over the temperature range from 37.2 K to 36.9 K in susceptometry mode, presenting the superconductivity develops in the scanned area. The diamagnetic signal starts to appear at 37.1 K at the bottom left corner of the scanned area, and then the top right corner. The whole area becomes superconducting at 36.9 K. The superconducting transition of the scanned area happens over the temperature range of 0.2 K.

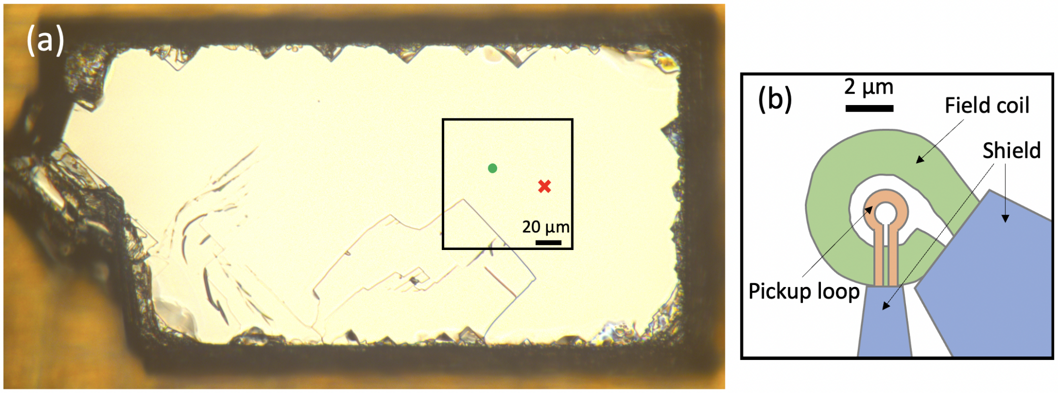


Figure S1: (a) Optical picture of the cleaved sample surface of $ab$ plane, with the scanned area of 100 $\mu$m $\times$ 100 $\mu$m marked as black box. The scale bar is 20 $\mu$m. The green circle shows the position for measuring the temperature dependent susceptibility in Figure 1a. The red cross shows the position for measuring the temperature dependent penetration depth and superfluid density in Figure 3. (b) Layout of the pickup-loop/field-coil geometry for the SQUID susceptometer. The inner diameter of pickup loop is 0.8 $\mu$m. The inner diameter of field coil is 3 $\mu$m. The pickup loop and field coil are encased in superconducting shields, leaving only the loop area exposed to detect local magnetic flux.

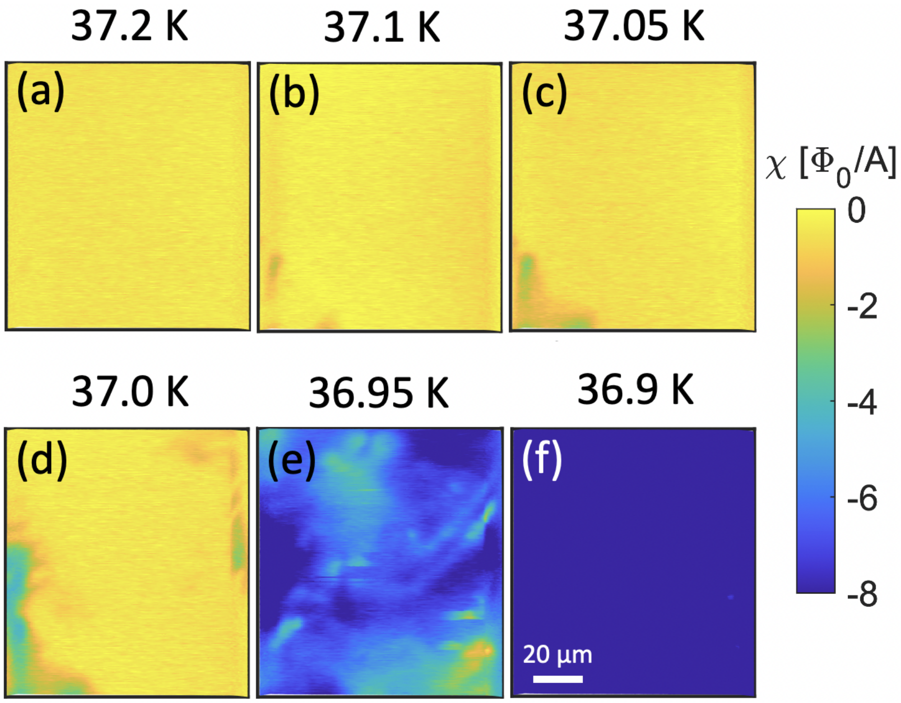


Figure S2: Susceptometry mode scans over the temperature range from 37.2 K to 36.9 K, showing the superconductivity develops in the scanned area. The background mutual inductance of the pick-up loop/field coil pair 17.7 $\Phi_0$/A is subtracted from all scans. The scale bar denotes 20 $\mu$m.

Figure S3a is measured at 25 K after cooling down from 40 K to 25 K, which is before the sample goes through the magnetic transition. After the sample is cooled down to the base temperature of 6.2 K and then warmed up though $T_m$ back to 25 K, the magnetometry scan is shown in Figure S3b. Comparing the two scans at 25 K in Figure S3, all the vortices remain the same positions. In addition, we checked the situation of higher vortex density with applying external magnetic field of 0.33 Gauss to generate more vortices in the same area. Same thing happened as illustrated Figure S4 that all the vortices were not rearranged through the magnetic transition.

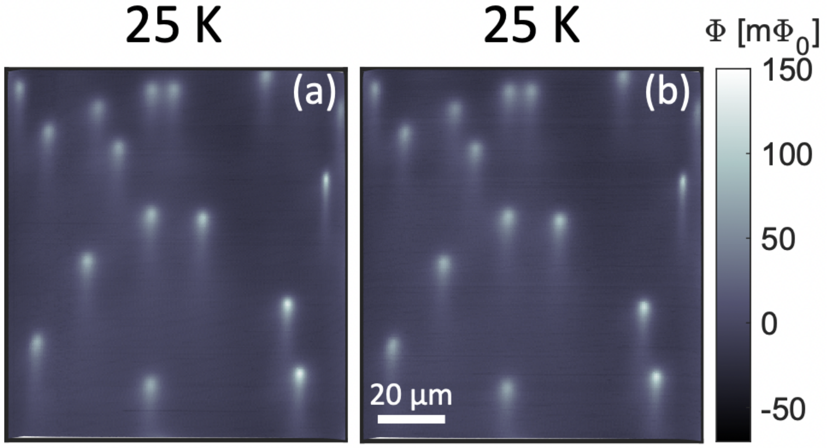


Figure S3: Two magnetometry scans at 25 K. (a) Scan at 25 K while cooling down from 40 K to 6.2 K. (b) Scan at 25 K while warming up from 6.2 K to 40 K. The vortices are not rearranged by comparing the two magnetometry scans.

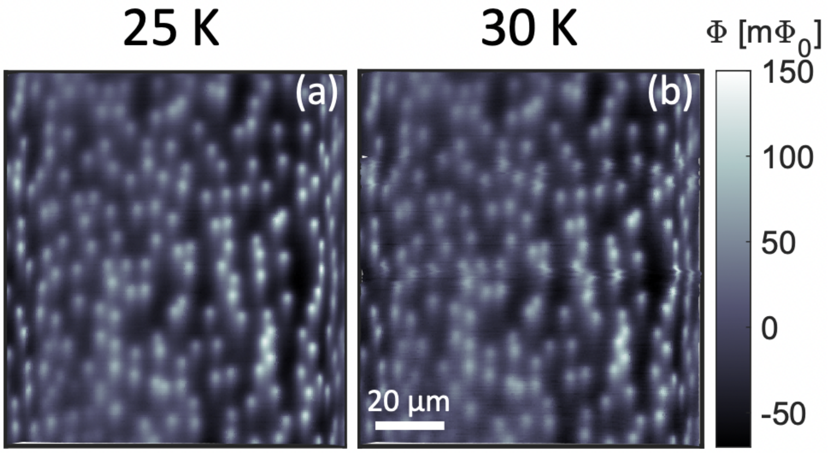


Figure S4: (a) Magnetometry scan at 25 K while cooling down from 50 K to 6.2 K. (b) Magnetometry scan at 30 K while warming up from 6.2 K to 40 K. The applied external magnetic field is 0.33 Gauss. All the vortices keep the same locations by comparing the two magnetometry scans.

## Supporting Note 2: Fitting method and procedure

We measured the susceptibility with the dependence of spacing from the sample surface to the SQUID sensor for different positions and temperatures. The measured susceptibility gets more diamagnetic when the sample moves towards the SQUID sensor. Because the spin configuration of $Eu^{2+}$ moments is in *ab* plane, and our measurements captured the out of *ab* plane component, we assume the contribution of paramagnetism from Eu layers to the measured susceptibility is not significant, and the measured susceptibility is from a bulk paramagnetic superconductor in the whole temperature range with predominantly diamagnetic response. By fitting the susceptibility as a function of spacing from the sample surface to the SQUID sensor, we can solve the London function and obtain the penetration depth.[1] We qualitatively discussed the effect of magnetism from local $Eu^{2+}$ moments on the penetration depth and superfluid density of the superconductivity in FeAs layers.

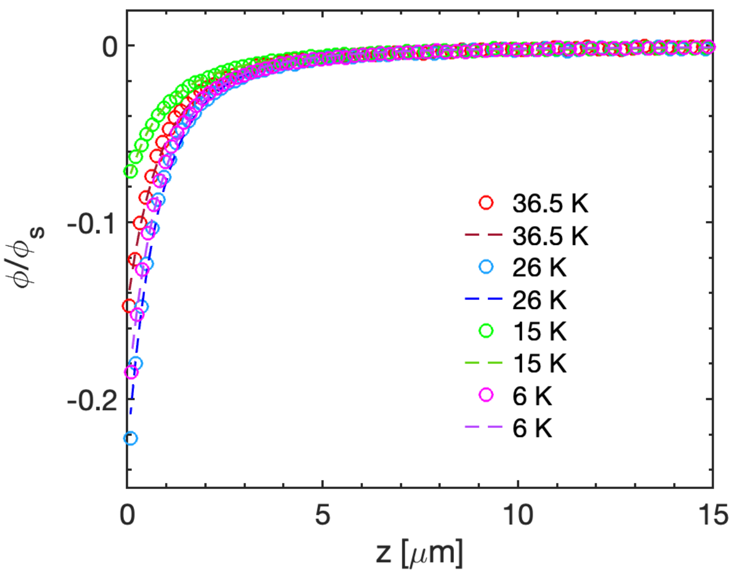


Figure S5: The normalized scanning SQUID susceptibility $\phi/\phi_s$ as a function of sample-sensor spacing $z$ at various temperatures. The circle symbols and dashed lines are the measured data and fits as described in the text.

The scanning SQUID measured susceptibility $\phi(z)$ as a function of sensor-sample spacing $z$ is given by

$$\phi(z)/\phi_s = \int_0^\infty dx\, x\, e^{-2x\bar{z}} J_1(x) \left[ \frac{-(\bar{q}+\bar{\mu}_2 x)(\bar{\mu}_3\bar{q}-\bar{\mu}_2 x) + e^{2\bar{q}\bar{t}}(\bar{q}-\bar{\mu}_2 x)(\bar{\mu}_3\bar{q}+\bar{\mu}_2 x)}{-(\bar{q}-\bar{\mu}_2 x)(\bar{\mu}_3\bar{q}-\bar{\mu}_2 x) + e^{2\bar{q}\bar{t}}(\bar{q}+\bar{\mu}_2 x)(\bar{\mu}_3\bar{q}+\bar{\mu}_2 x)} \right]. \quad (1)$$

In Eq.1, $\phi_s$ is the field-coil to pickup loop mutual inductance in $\Phi_0$/A. $\bar{z} = z/a$, where $a$ is the field coil effective radius. $J_1$ is Bessel function. $\bar{\mu}_2$ and $\bar{\mu}_3$ are the permeability of the sample and sample stage divided by that of vacuum $\mu_0$. Here we assume $\bar{\mu}_2 = 1$ and $\bar{\mu}_3 = 1$ for simplicity. $\bar{q} = \sqrt{x^2 + 1/\bar{\lambda}^2}$, where $\bar{\lambda} = \lambda/a$. $\bar{t} = t/a$, where $t$ is the sample thickness.

When the sample surface touches the SQUID sensor defined as $z = 0$, the pickup loop center locates at a height of $z_0$ depending on the SQUID sensor geometry and the angle between the SQUID chip and the sample surface. In the fittings, we assume $z_0 = 1.2$ $\mu$m. With the assumptions, the fitted London penetration depth at 6 K is 0.568(6) $\mu$m which is a reasonable value comparing with the previous study of optical conductivity measurements with evaluated $\lambda \sim (420 \pm 45)$ nm at 4 K,[2] also comparable to the similar iron pnictides.

Figure S5 shows the measured data and fits for the normalized scanning SQUID susceptibility $\phi/\phi_s$ as a function of sample-sensor spacing $z$ at various temperatures. The fittings describe the data very well, yielding the London penetration depth $\lambda$.

## Supporting Note 3: Video captions

Video S1. Video of the temperature dependent susceptometry and magnetometry scans.

## Supporting Note 4: Weak $c$-axis magnetization

To clarify the weak $c$-axis magnetization, we performed a calculation to estimate the resulting magnetic flux from the full effective moment of Eu spins. Given the effective moment of Eu as 7.94 $\mu_B$/Eu, calculated by $\mu_{eff} = g\mu_B\sqrt{S(S+1)}$ with $g = 2$ and $S = 7/2$, we deduced a magnetic field of $\sim$ 0.46 T using $B = \mu_0 M = \mu_0\,\rho\,\mu_{eff}$, where $\rho$ denotes the density of magnetic ions. Considering the dimensions of our pickup loop, this magnetic field (0.46 T) corresponds to $\sim 112\ \Phi_0$, where $\Phi_0$ represents the magnetic flux quantum. With the pickup loop placed $\sim 1\ \mu$m above the sample surface, the resulting magnetic flux captured by our pickup loop is estimated to be $\sim 30\ \Phi_0$ using $B_z \propto B_{z=0} \cdot e^{-kz}$, where $z$ is the spacing between the pickup loop and sample surface. This magnitude ($\sim 30\ \Phi_0$) is much larger than the color bar range of our magnetometry scans spanning 0.1 $\Phi_0$, suggesting that the magnetic domains we observed harbor a considerably weak ferromagnetic component.

## Supporting Note 5: Scanning SQUID's point spread function

Scanning SQUID magnetometry images include the effect of the point spread function (PSF) of the SQUID.[3] In our configuration, the PSF $g$ has an asymmetric structure [Figure S6(a)].

To obtain this PSF, we used a magnetometry scan over an isolated vortex (not shown) and the magnetic point source model describing the out-of-plane component of the magnetic field $B_z(x, y, z) = \Phi_0(z + \lambda)/[x^2 + y^2 + (z + \lambda)^2]^{3/2}$, where a magnetic monopole with the flux quantum $\Phi_0$ is placed at $x = y = z = 0$, the scan height $z = 1068$ nm, the penetration depth $\lambda = 453.5$ nm at 25 K. From the observed magnetometry scan $\Phi$, we calculate $B_z$ as $IFFT[H * FFT[\Phi]/FFT[g]]$, where $H$ is the Hanning filter (low-pass filter) and FFT(IFFT) is (Inverse) Fast Fourier Transformation for the discrete data. The calculated $B_z$ has the point source magnetic field as we expect and the "tail" features almost disappear. Note that there are oscillating backgrounds with weak amplitude, which originate from the experimental noise in the original magnetometry data that we used to create the PSF $g$. Similar backgrounds are seen in the PSF.

This calculation was also applied to the measured data in Figure 2(a). The "tail" features are successfully removed from the vortex fields [Figure S7]. Importantly, the magnetic domains in $B_z$ exhibit similar magnetic structures as those in the $\Phi$ images, indicating that our discussion of the spatial structure of magnetic domains based on the $\Phi$ images in the main text remain unaffected, ensuring the reliability and accuracy of our interpretation and conclusion.

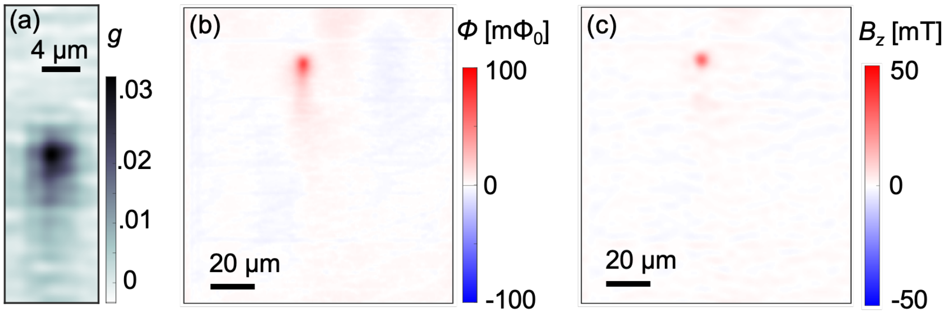


Figure S6: Asymmetric point spread function of SQUID produces the weak "tail" feature. (a) SQUID's point spread function. (b) Magnetometry scan with an isolated vortex at 25 K. (c) Out of plane component of the calculated magnetic field $B_z$ using (a) and (b).

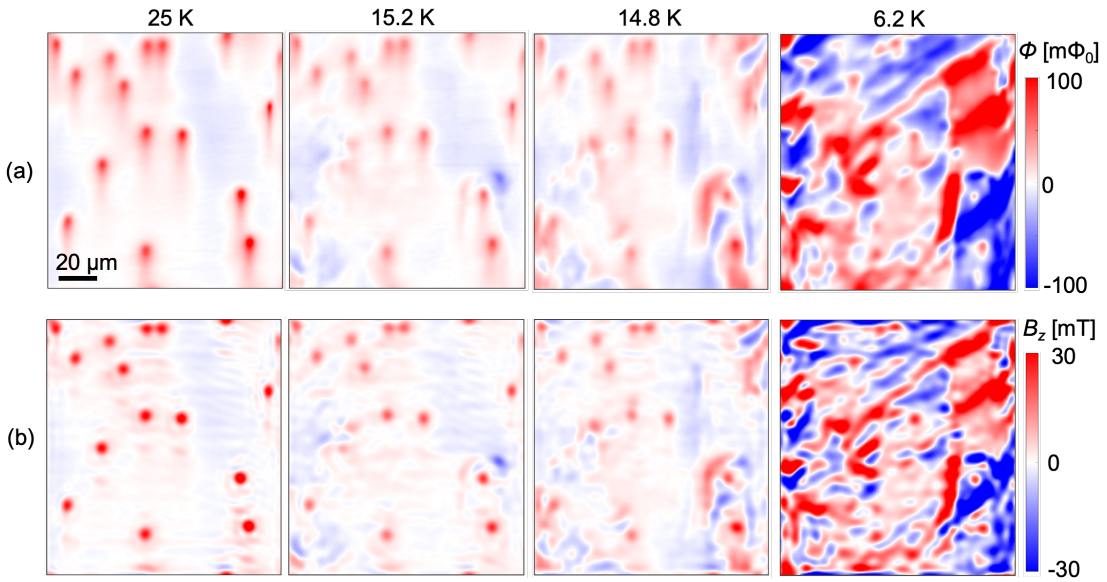


Figure S7: Calculated magnetic field exhibits similar magnetic structures to flux scans incorporating SQUID's asymmetric point spread function. (a) The observed magnetic flux scan, copied from Figure 2(a). (b) The calculated $B_z$ from (a) with Figure S6(a). Data exceeding the color plot's maximum (minimum) are plotted with the same color as the maximum (minimum) value to make the more important smaller values easier to see.

# References


(1) Kirtley, J. R.; Kalisky, B.; Bert, J. A.; Bell, C.; Kim, M.; Hikita, Y.; Hwang, H. Y.; Ngai, J. H.; Segal, Y.; Walker, F. J.; Ahn, C. H.; Moler, K. A. Scanning SQUID susceptometry of a paramagnetic superconductor. *Phys. Rev. B* **2012**, *85*, 224518.

(2) Stolyarov, V. S.; Casano, A.; Belyanchikov, M. A.; Astrakhantseva, A. S.; Grebenchuk, S. Y.; Baranov, D. S.; Golovchanskiy, I. A.; Voloshenko, I.; Zhukova, E. S.; Gorshunov, B. P.; Muratov, A. V.; Dremov, V. V.; Vinnikov, L. Y.; Roditchev, D.; Liu, Y.; Cao, G.-H.; Dressel, M.; Uykur, E. Unique interplay between superconducting and ferromagnetic orders in $EuRbFe_4As_4$. *Phys. Rev. B* **2018**, *98*, 140506(R).

(3) Spanton, E. M. Imaging current in materials. *Ph.D. thesis* **2016**, Stanford University.
